# Supplementary material for: Comparing large language models for supervised analysis of students' lab notes
Source: arXiv:2412.10610 source file (2025-02-24)
Supplement: Supplementary file 1 [file appendix.tex]

Given a labeled test set of size N, we measure the model output on the data and calculate a confusion matrix given by Table \ref{confusion}:

\begin{table}
\caption{The confusion matrix}\label{confusion}
\begin{tabular}{l|l|c|c|}
\multicolumn{2}{c}{}&\multicolumn{2}{c}{Human coder}\\
\cline{3-4}
\multicolumn{2}{c|}{}&Positive&Negative\\
\cline{2-4}
\multirow{2}{*}{Model}& Positive & $TP$ & $FP$\\
\cline{2-4}
& Negative & $FN$ & $TN$\\
\cline{2-4}
\end{tabular}
\end{table}

Where $TP$, $FP$, $FN$ and $TN$ stand for: True Positive, False Positive, False Negative and True Negative respectively, where we consider the model to be accurate when it agrees with a human coder.

If we now use the model on a new set of sentences, a human coder would believe a percentage of the new sentences, $E_H$ contain the code.

Given this, we expect our machine classifier to measure the percentage of the sentences as containing the code ($E_c$) to be:  

\begin{equation}
    E_c = E_H P_{TPP} +(1-E_H)*P_{FPN}
    \label{ec}
\end{equation}

In words, this is:  The measured ratio of sentence containing the code will be equal to the probability that a randomly selected sentence contains the code times the probability that a sentence that contains the code is classified correctly by the classifier ($P_{TPP}$), plus the probability that a sentence that does not contain the code is incorrectly classified by the classifier ($P_{FPN}$)

Here, we make the assumption that the probability that a sentence is misclassified (given that it does or does not contain the code) does not change given a different proportion of sentences containing the code in the dataset.

We can calculate these probabilities from the confusion matrix:  

\begin{equation}
    P_{TPP}= \frac{TP}{TP+FN}
\end{equation}

\begin{equation}
    P_{FPN}= \frac{FP}{FP+TN}
\end{equation}

We solve equation \ref{ec} for $E_H$, and find: 
\begin{equation}
    E_H=\frac{E_C-P_{FPN}}{P_{TPP}-P_{FPN}}
\end{equation}

If we want the expected error, we can plug in:  
\begin{equation}
    S=E_C-E_H=E_C-\frac{E_C-P_{FPN}}{P_{TPP}-P_{FPN}}
\end{equation}
or 
\begin{equation}
    S=E_C(1-\frac{1}{P_{TPP}-P_{FPN}})+\frac{P_{FPN}}{P_{TPP}-P_{FPN}}
\end{equation}
